# Supplementary material for: Gouy phase-matched angular and radial mode conversion in four-wave mixing
Source: arXiv:2007.14125 ancillary file (2021-02-25)
Supplement: Supplementary file 1 [file P_mode__Supplementary_material_.pdf]

# Gouy phase-matched angular and radial mode conversion in four-wave mixing: supplementary material

Rachel F. Offer, Andrew Daffurn, Erling Riis, Paul F. Griffin, and Aidan S. Arnold
*Department of Physics, SUPA, University of Strathclyde, Glasgow G4 0NG, UK*

Sonja Franke-Arnold
*School of Physics and Astronomy, SUPA, University of Glasgow, Glasgow G12 8QQ, UK*
(Dated: February 25, 2021)

Further details on our paper are provided here, comprising three sections on: the theoretical model; the experimental details; the supporting results and figures.

## S1. THEORETICAL MODEL

The electric field of the Laguerre-Gauss modes is given in cylindrical polar coordinates by

$$\mathrm{LG}_p^\ell(r,\theta,z) = \sqrt{\tfrac{2p!}{\pi(|\ell|+p)!}}\tfrac{1}{w(z)}\left(\tfrac{\sqrt{2}r}{w(z)}\right)^{|\ell|} e^{-\frac{r^2}{w(z)^2}} \times L_p^{|\ell|}\left(\tfrac{2r^2}{w(z)^2}\right) e^{i\Phi_\mathrm{C}(z,r)}\, e^{i\Phi_\mathrm{G}(z)}\, e^{i\ell\theta}, \quad \text{(S1)}$$

where $L_p^{|\ell|}$ is a Laguerre polynominal. The beam radius varies with propagation according to $w(z) = w_0\sqrt{1+z^2/z_R^2}$, for beam waist $w_0$ and Rayleigh range $z_R = \pi w_0^2/\lambda$. The phase $\Phi_\mathrm{C} = k\left(z+\frac{r^2}{2}(z+z_\mathrm{R}{}^2/z)^{-1}\right)$ accounts for wavefront curvature and $\Phi_\mathrm{G} = -N_p^\ell \arctan(z/z_\mathrm{R})$ is the Gouy phase, where $N_p^\ell = 1+2p+|\ell|$ is the mode order.

For given 780 nm and 776 nm pump modes, the 3D overlap integral over the cell length $L$ allows us to predict the (root) relative probability of generating a particular pair of blue and infrared FWM modes as:

$$c_{p_\mathrm{B},p_\mathrm{IR}}^{\ell_\mathrm{B},\ell_\mathrm{IR}} = \int_{-L/2}^{L/2} dz \int_0^{2\pi} d\theta \int_0^\infty dr\, r\, \mathrm{LG}_{\mathrm{p}_{780}}^{\ell_{780}}\, \mathrm{LG}_{\mathrm{p}_{776}}^{\ell_{776}}\, \mathrm{LG}_{\mathrm{p}_\mathrm{IR}}^{\ell_\mathrm{IR}*}\, \mathrm{LG}_{\mathrm{p}_\mathrm{B}}^{\ell_\mathrm{B}*}, \quad \text{(S2)}$$

equivalent to Eq. 1 in the main paper.

This integral requires the appropriate beam waist for each field. The 780 nm and 776 nm waists are set by their measured experimental value $w_0$. The blue and infrared waists are then chosen such that their Rayleigh ranges match the pump fields: $w_\mathrm{B} = (\frac{420}{780})^{1/2} w_0$, $w_\mathrm{IR} = (\frac{5230}{780})^{1/2} w_0$. This is an extension of the Boyd criterion [1], which states that wave mixing with Gaussian beams in an extended nonlinear medium is maximally efficient when the fields have matched Rayleigh ranges.

In general, both the infrared and blue FWM fields may be generated in a range of modes. The 420 nm mode superposition for a given IR mode is then:

$$u_\mathrm{B}^{\ell_\mathrm{IR},p_\mathrm{IR}} = \sum_{p_\mathrm{B}} c_{p_\mathrm{B},p_\mathrm{IR}}^{\ell_\mathrm{B},\ell_\mathrm{IR}} \mathrm{LG}_{p_\mathrm{B}}^{\ell_\mathrm{B}} = \sum_{p_\mathrm{B}} c_{p_\mathrm{B},p_\mathrm{IR}}^{\ell_\mathrm{T}-\ell_\mathrm{IR},\ell_\mathrm{IR}} \mathrm{LG}_{p_\mathrm{B}}^{\ell_\mathrm{T}-\ell_\mathrm{IR}}, \quad \text{(S3)}$$

where for the final expression we have used the fact that OAM is conserved, i.e. $\ell_{780}+\ell_{776} = \ell_\mathrm{T} = \ell_\mathrm{B}+\ell_\mathrm{IR}$. However, especially in thick media, agreement with experiment is best when we only consider 420 nm modes generated for Gaussian IR, so that $\ell_\mathrm{B} = \ell_\mathrm{T}$, with the blue light generated in a coherent superposition of radial modes, with complex coefficients given by the overlap integral Eq. S2:

$$u_\mathrm{B}(r,\theta,z) = \sum_{\ell_\mathrm{T},p_\mathrm{B}} c_{p_\mathrm{B},0}^{\ell_\mathrm{T},0}\, \mathrm{LG}_{p_\mathrm{B}}^{\ell_\mathrm{T}}(r,\theta,z). \quad \text{(S4)}$$

We calculate predicted beam profiles by evaluating $|u_\mathrm{B}(r,\theta,z)|^2$ at $z=0$ for the near field and $z \gg z_\mathrm{R}$ for the far field.

The values of $c_{p_\mathrm{B},0}^{\ell_\mathrm{T},0}$ critically depend on the relative length of the Rayleigh range and the nonlinear medium. In the thin crystal limit (large $z_\mathrm{R}/L$) there is little axial variation of the fields, thus $p$-modes which produce good radial overlap with the pump beams are generated. In contrast, in an extended medium (small $z_\mathrm{R}/L$) the axial propagation is crucial. Modes which do not conserve mode order undergo a Gouy phase shift relative to the pump beams, and are thus suppressed. In the thick medium limit only modes which obey

$$(N_p^\ell)_{780} + (N_p^\ell)_{776} = (N_p^\ell)_\mathrm{IR} + (N_p^\ell)_\mathrm{B} \quad \text{(S5)}$$

are generated. For Gaussian IR, this means $u_\mathrm{B} = \mathrm{LG}_{p_\mathrm{B}}^{\ell_\mathrm{T}}$, where $p_\mathrm{B} = p_{780}+p_{776}+(|\ell_{780}|+|\ell_{776}|-|\ell_\mathrm{T}|)/2$.

In the main text we experimentally demonstrate two important phenomena which follow from this. Firstly, for $|\ell_{780}|+|\ell_{776}| > |\ell_\mathrm{T}|$ (main paper Fig. 2 (c,e) and Fig. 3 right two images) we observe angular-to-radial mode conversion – i.e. $p_\mathrm{B} > p_{780}+p_{776}$. Secondly, for $|\ell_{780}|+|\ell_{776}| = |\ell_\mathrm{T}|$ (main paper Fig. 4(c,e) and Fig. 5) we have $p_\mathrm{B} = p_{780}+p_{776}$ – i.e. we observe addition of input radial indices.

The tilted lens interference patterns are simulated by multiplying $u_\mathrm{B}(x,y,z \gg z_\mathrm{R})$ with a spatially varying phase shift

$$\phi_\mathrm{TL}(x,y) = \exp\left[-ik\left[\frac{(x-x_0)^2}{2f/\cos\theta} + \frac{(y-y_0)^2}{2f\cos\theta}\right]\right], \quad \text{(S6)}$$

where $f$ and $\theta$ are the focal length and angle of the lens, respectively, and then carrying out a numerical plane wave decomposition to propagate the resulting field to the lens focus.

We now come back to our initial model: if the IR field is no longer constrained to a Gaussian, Eq. S3 holds, and the blue beam is generated as a coherent superposition of radial modes which conserve OAM. Assuming the FWM process is purely spontaneous, the total blue light intensity is then the incoherent sum over all IR modes [2, 3]:

$$|u_{\mathrm{B}}|^2 = \sum_{\ell_{\mathrm{IR}},p_{\mathrm{IR}}} |u_{\mathrm{B}}^{\ell_{\mathrm{IR}},p_{\mathrm{IR}}}|^2.$$

We note that in previous thick medium work [4], with $|\ell_{780}| + |\ell_{776}| = |\ell_{\mathrm{T}}|$ and $p_{780} = p_{776} = 0$, we found good agreement with this model, specifically for larger values of OAM. It remains unclear why this is not the case for the more general mode mixing presented here, but we assume that this would be explained by a more complete model including absorption and dispersion upon propagation, as well as stimulated processes. This is particularly important for processes affecting individual modes differently. For example saturated absorption and Kerr lensing may have more of an effect for modes with greater local intensity variation (e.g. modes with $p > 0$). Stimulated wave mixing processes would act to increase the relative power in the most probable IR and blue mode pair, and may partly explain the apparent favouring of the IR $\mathrm{LG}_0^0$ mode.

## S2. EXPERIMENTAL DETAILS

In this section we include additional details of our experimental setup. The pump beams are provided by extended cavity diode lasers (ECDLs [5]) at 780 nm and 776 nm. The lasers are locked to appropriate hyperfine transitions via DAVLL [6] and two-photon spectroscopy, respectively. Laser detunings are chosen to minimise Kerr lensing [4]: the 780 nm laser is locked approximately halfway between the $^{85}$Rb ground states, i.e. 1.52 GHz blue of the $5S_{1/2}\,F = 3 \to 5P_{3/2}\,F' = 4$ transition, with the 776 nm laser two-photon resonant with the $5S_{1/2}\,F = 3 \to 5D_{5/2}\,F' = 5$ transition.

After beam shaping, the LG pump mode powers are $\approx 1$ mW before entering the 120 °C [7] Rb cell. The pump power is limited by the use of a non-polarising beamsplitter to combine the 780 nm and 776 nm pump light, as well as losses at the spatial light modulator (SLM). We work deliberately at low SLM efficiency to enable rapid variation of $\ell$ for fixed waist $w$, as light for $p = 0$ modes (Eq. S1) is mainly diffracted from an annular region of radial width $w$ with mean radius $(\ell/2)^{1/2}w$. However, we note higher efficiencies could be achieved with more SLMs/SLM sub-section interactions [8], permitting decoupling between final beam size $w$ and the $p$, $\ell$ indices.

## S3. SUPPORTING RESULTS

In this section we include the full experimental results of measurements mentioned in the main text.

Fig. S1 illustrates a gradual variation of medium thickness under the same FWM conditions as Fig. 2 in the paper, i.e. for pump modes $u_{780} = \mathrm{LG}_0^1$ and $u_{776} = \mathrm{LG}_0^{-1}$. We vary the inverse thickness parameter between 0.49 and 1.03 by adjusting the waists of the pump beams for a fixed cell length. The observed beam profiles show a

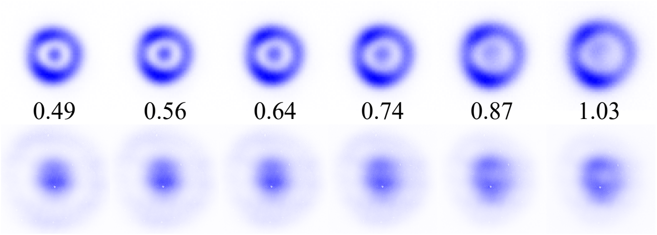


FIG. S1. Observed near- (upper) and far-field (lower) 420 nm transverse profiles resulting from pump beams $u_{780} = \mathrm{LG}_0^1$ and $u_{776} = \mathrm{LG}_0^{-1}$, as $z_{\mathrm{R}}/L$ (labelled) varies.

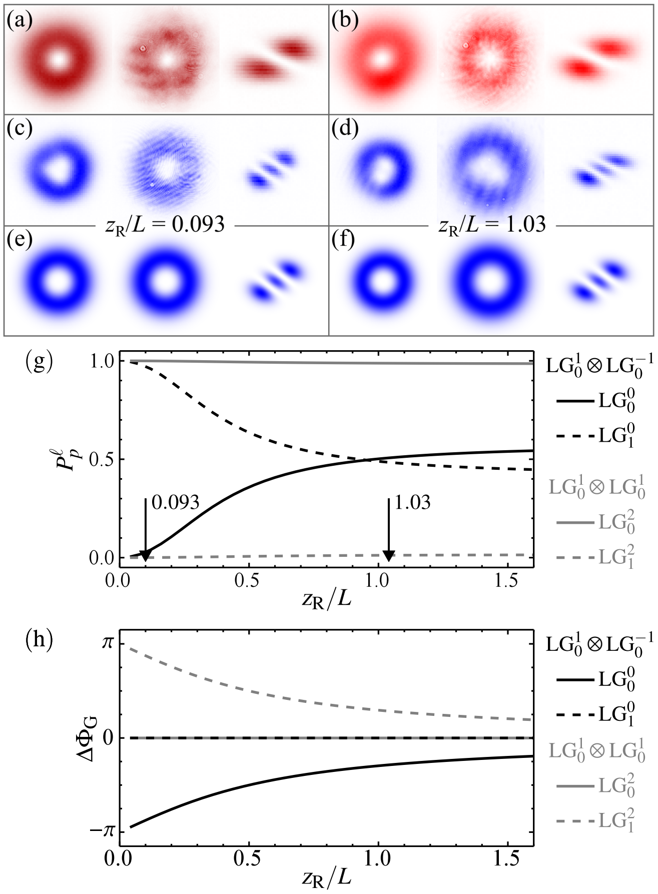


FIG. S2. FWM for pump modes with *equal* $\ell$, i.e. $u_{780} = \mathrm{LG}_0^1$ (a) and $u_{776} = \mathrm{LG}_0^1$ (b). All other parameters are the same as in Fig. 2 of the main paper, with the equivalent meanings within each image triplet (c)-(f). The corresponding theoretical relative mode powers and integrated Gouy phase mismatch as a function of inverse medium thickness are shown in (g) and (h), respectively, for pump modes with equal (grey) and opposite (black) OAM.

varying decomposition of $\mathrm{LG}_0^0$ and $\mathrm{LG}_1^0$.

Fig. S2 shows FWM complementary to Fig. 2 in the main paper, i.e. for identical pump modes $u_{780} = u_{776} = \mathrm{LG}_0^1$, with the same OAM. The individual pump beam intensities coincide with those in Fig. 2, but total OAM conservation in FWM results in markedly different blue light modes. Fig. S2 (c) and (d) show $u_\mathrm{B} = \mathrm{LG}_0^2$ is generated, independent of the medium thickness, agreeing with previous experimental observations [4, 9, 10]. The matching theory profiles are calculated by constraining the IR field to $\mathrm{LG}_0^0$ like in the main text, however similar agreement is also found without this constraint.

Mode decomposition varies with medium thickness for pump beams with opposite OAM (Fig. 2 and black curves in Fig. S2 (g)), but remains constant for equal OAM (Fig. S2(a-f) and grey curves in (g)). The independence on medium thickness in the latter case can be explained by considering the Gouy phases of the individual modes.

Fig. S2 (h) shows the integrated Gouy phase mismatch $\Delta\Phi_\mathrm{G}$ for different blue modes, as a function of the inverse thickness parameter. We define this phase mismatch as:

$$\Delta\Phi_\mathrm{G} = \frac{1}{L}\int_{-L/2}^{L/2} [\delta\Phi_\mathrm{G}(z) - \delta\Phi_\mathrm{G}(-L/2)]\, dz, \qquad \text{(S7)}$$

where $\delta\Phi_\mathrm{G}(z) = \Phi_\mathrm{G}^{780}(z) + \Phi_\mathrm{G}^{776}(z) - \Phi_\mathrm{G}^{\mathrm{IR}}(z) - \Phi_\mathrm{G}^{\mathrm{B}}(z)$. In a thin medium (large $z_\mathrm{R}/L$) the accumulated phase mismatch is small and Gouy phase matching has little effect – any OAM-conserving modes which have good spatial overlap with the pump beams are generated. For increasing medium thickness the phase mismatch increases for mode combinations which do not conserve mode order, thus suppressing these modes. For mode combinations which conserve mode order, e.g. for $u_{780}\, u_{776}\, u_\mathrm{IR}^*\, u_\mathrm{B}^* = \mathrm{LG}_0^1\, \mathrm{LG}_0^{-1}\, \mathrm{LG}_0^{0*}\, \mathrm{LG}_1^{0*}$ and $\mathrm{LG}_0^1\, \mathrm{LG}_0^1\, \mathrm{LG}_0^{0*}\, \mathrm{LG}_0^{2*}$, the phase mismatch $\Delta\Phi_\mathrm{G}$ is zero irrespective of $z_\mathrm{R}/L$.

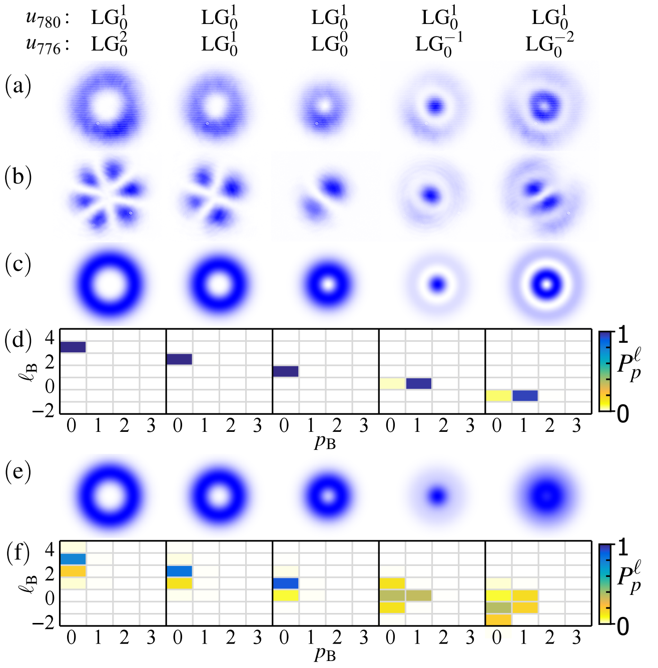


FIG. S3. Angular-to-angular and angular-to-radial mode conversion for FWM of $u_{780} \otimes u_{776} = \mathrm{LG}_0^1 \otimes \mathrm{LG}_0^{\ell_{776}}$ input beams in the 'thick medium' regime. (a) Resulting blue beam profiles in the far field, and (b) interferogram. Predicted beam profile (c) and normalised mode powers (d) for $u_\mathrm{IF} = \mathrm{LG}_0^0$, and for a wider range of IR modes with $-2 \leq \ell_\mathrm{IR} \leq 2$ and $0 \leq p =\leq 3$ in (e) and (f).

All subsequent results were taken in the thick medium regime. We observe two effects: angular-to-radial mode conversion for pump beams with oppositely signed OAM, and addition of radial indices for pump beams with $p > 0$.

Fig. S3 expands on the results of Fig. 3 in the main paper, with the same experimental conditions: $u_{780} = \mathrm{LG}_0^1$ and $u_{776} = \mathrm{LG}_0^{\ell_{776}}$ for $-2 \leq \ell_{776} \leq 2$. We further note that the modal decompositions for FWM from $u_{780}\, u_{776} = \mathrm{LG}_0^1\, \mathrm{LG}_0^1$ and $\mathrm{LG}_0^1\, \mathrm{LG}_0^{-1}$ apply to the thick medium results in Fig. S2 and Fig. 2, respectively.

Fig. S3 (a) shows the $u_\mathrm{B}$ far-field beam profiles, demonstrating angular-to-radial mode conversion when $\ell_{776} < 0$, generating blue light with $p_\mathrm{B} = 1$. In Fig. S3 (b) we use Dove-prism interferometry to investigate the phase structure. The characteristic patterns, formed by interfering the beam with its mirror image, have $2|\ell_\mathrm{B}|$-fold rotational symmetry. Although this method is insensitive to the sign of $\ell_\mathrm{B}$, we observe $|\ell_\mathrm{B}| = |\ell_\mathrm{T}| = |1 + \ell_{776}|$ as expected from OAM conservation for $u_\mathrm{IR} = \mathrm{LG}_0^0$.

Fig. S3 (c) and (d) show the theoretical beam profiles and relative power in each 420 nm mode, again assuming $u_\mathrm{IR} = \mathrm{LG}_0^0$, which agree well with the experimental results. In contrast, (e) and (f) show the equivalent results without constraining $u_\mathrm{IR}$, where the model clearly breaks down for $\ell_{776} < 0$. For $\ell_{776} \geq 0$ both theory approaches lead to similar results, in the unconstrained theory the dominant $u_\mathrm{B}$ mode is paired with $u_\mathrm{IR} = \mathrm{LG}_0^0$, and as a result restricting the IR to $\mathrm{LG}_0^0$ has only a small effect. In contrast, for $\ell_{776} < 0$ the two theories give very different results, with only the constrained model agreeing with our experimental observations.

Finally, we provide additional experimental and theoretical information related to Fig. 5 in the main text, demonstrating the generation of higher order radial

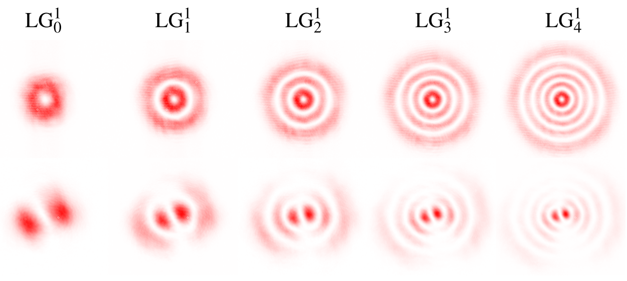


FIG. S4. Example beam profiles and interferograms of the $u_{780}$ pump beam for $\ell_{780} = 1$ and $0 \leq p_{780} \leq 4$.

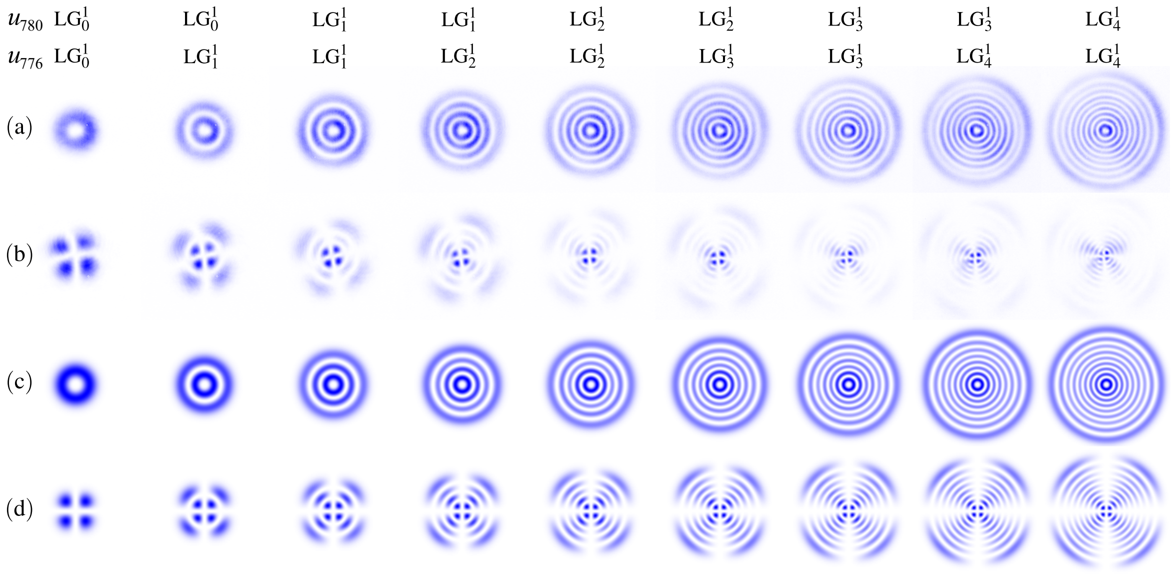


FIG. S5. Normalised far-field 420 nm intensity profile (a) and interferogram (b) for $p$-mode 'additions' using a variety of $\mathrm{LG}^1_{p_{780}}$ and $\mathrm{LG}^1_{p_{776}}$ pump modes. Predicted intensity profile (c) and interferograms (d) assuming $u_{\mathrm{IR}} = \mathrm{LG}^0_0$.

modes $u_{\mathrm{B}} = \mathrm{LG}^2_p$, where $p$ takes all values from 0 to 8. We achieve this by combining a variety of pump modes $u_{780} = \mathrm{LG}^1_{p_{780}}$ and $u_{776} = \mathrm{LG}^1_{p_{776}}$, where $0 \leq p_{780} \leq 4$ and $0 \leq p_{776} \leq 4$. Fig. S4 shows the corresponding $u_{780}$ beam profiles. The high visibility interferograms with two lobes indicate $|\ell| = 1$ with high purity. Close inspection reveals a slight difference in the radial profile of the beam profile images, taken in the image plane of the SLM, and the interferograms, taken after some propagation, indicating minor contamination of the radial mode by a weak additional coherent $p$ contribution.

Fig. S5 shows the corresponding generated blue light, reproducing the beam profiles (Fig. 5 main text) in (a), as well as the associated interferograms (b), with simulated profiles and interferograms in (c) and (d). The beam profiles demonstrate clean conversion of the radial pump indices, with $p_{\mathrm{B}} = p_{780} + p_{776}$ nodal rings. Each interferogram shows high visibility fringes, with 4 lobes, indicating that $|\ell| = 2$, independent of the pump $p$ index. We note a minor change in radial profile between the beam profile and interferogram images, which, like the pump mode results in Fig. S4, were taken at different propagation distances. This may be entirely due to the slight pump mode contamination evident in Fig. S4, or there may be additional loss of purity from the FWM process. In all cases, the dominant mode remains $p_{\mathrm{B}} = p_{780} + p_{776}$. The simulated beam profiles and interferograms in (c) and (d), were calculated under the assumption of $u_{\mathrm{IR}} = \mathrm{LG}^0_0$, and for $p_{\mathrm{B}} = 0 \to 10$. In each case the relative power in the mode with $p_{\mathrm{B}} = p_{780} + p_{776}$ was $> 98\%$. This high mode purity demonstrates the critical effect of Gouy phase matching in the thick medium regime.


[1] G. D. Boyd and D. A. Kleinman, J. Appl. Phys. **39**, 3597 (1968).

[2] A. Mair, A. Vaziri, G. Weihs, and A. Zeilinger, Nature **412**, 313 (2001).

[3] R. N. Lanning, Z. Xiao, M. Zhang, I. Novikova, E. E. Mikhailov, and J. P. Dowling, Phys. Rev. A **96**, 013830 (2017).

[4] R. F. Offer, D. Stulga, E. Riis, S. Franke-Arnold, and A. S. Arnold, Commun. Phys. **1**, 84 (2018).

[5] A. S. Arnold, J. S. Wilson, and M. G. Boshier, Rev. Sci. Instrum. **69**, 1236 (1998).

[6] K. L. Corwin, Z. T. Lu, C. F. Hand, R. J. Epstein, and C. E. Wieman, Appl. Opt. **37**, 3295 (1998).

[7] P. Siddons, C. S. Adams, C. Ge, and I. G. Hughes, J. Phys. B **41**, 155004 (2008).

[8] S. Scholes, V. Rodríguez-Fajardo, and A. Forbes, arXiv:2004.10196 (2020).

[9] A. M. Akulshin, I. Novikova, E. E. Mikhailov, S. A. Suslov, and R. J. McLean, Opt. Lett. **41**, 1146 (2016).

[10] A. Chopinaud, M. Jacquey, B. Viaris de Lesegno, and L. Pruvost, Phys. Rev. A **97**, 063806 (2018).
